# Supplementary material for: DiaQ: Efficient State-Vector Quantum Simulation
Source: arXiv:2405.01250 source file (2024-04-30)
Supplement: Supplementary file 1 [file 13-appendix.tex]

\clearpage

\twocolumn[%
{\centering\huge{Appendix: Artifact Description \\[1em]}}
]

\section*{\large\textbf{Summary of the experiments reported}}
We conducted experiments using the SV-Sim simulator with and without libdiaq integration. The benchmarks used were from SupermarQ and QASMbench. The experiments were performed on Intel's Broadwell processor using gcc-12.3, cmake-3.26.5, and OLCF's Frontier processor using gcc-12.2, cmake-3.20.4. The paper presents three major contributions: 1) The formulation of the DiaQ format and the implementation of the libdiaq C++ library with OpenMP multi-threading and SIMD vectorization, 2) The integration of libdiaq with SV-Sim, and 3) The evaluation plots. The following artifacts provide detailed information on each of these contributions (\href{https://drive.google.com/file/d/1P4Ts8rzcr8S0QYRUToQfzNaBemktPi8g/view?usp=share_link}{Private link to our artifacts on Google Drive}).

\begin{lstlisting}[frame=single, basicstyle=\small\ttfamily, breaklines=true]
# download all the artifacts (diaq_sc24.zip)
$ wget --content-disposition "https://drive.usercontent.google.com/download?id=1P4Ts8rzcr8S0QYRUToQfzNaBemktPi8g&export=download&confirm=t&uuid=e893fa5a-9c33-4c24-baf9-b7a00b8b3a27" --no-check-certificate
$ unzip diaq_sc24.zip && cd diaq_sc24
\end{lstlisting}

\textbf{1) The DiaQ C++ library:}
The \texttt{libdiaq} library is implemented with SIMD and OpenMP multi-threading. It requires cmake $\geq$ 3 and gcc $\geq$ 12, g++ $\geq$ 12 as prerequisites. The following steps outline the build and testing process:

\begin{lstlisting}[frame=single, basicstyle=\small\ttfamily, breaklines=true]
$ cd diaq
$ mkdir build && cd build
$ cmake .. && make -j 4 && cd ..
# run 48 spGEMM tests
$ ./build/bin/tests
# run spMV test
$ ./build/bin/tests spmv_1
# optionally install diaq as a python library
$ pip install --no-cache-dir .
# run numpy to diaq test
$ python tests/conversion_test.py
\end{lstlisting}

\textbf{2) NWQ-Sim library:}
The NWQ-Sim library source code from PNNL includes additional "backends" for SV-Sim + DiaQ integrations. The prerequisites for building and testing include cmake $\geq$ 3, gcc $\geq$ 12, g++ $\geq$ 12, and libdiaq installed. The following steps outline the process:

\begin{lstlisting}[frame=single, basicstyle=\small\ttfamily, breaklines=true]
$ cd NWQ-Sim
# build default SV-Sim
$ mkdir build_w_dense && cd build_w_dense
$ cmake -DCUDA_ARCH=75 .. && make -j 4
# sanity check the normal build
$ ./qasm/nwq_qasm -q ../data/benchmarks/ghz/ghz22.qasm -backend OpenMP -sim sv -metrics
# build SV-Sim with libdiaq integrations
$ cd .. && mkdir build_w_diaq && cd build_w_diaq
$ cmake -DCUDA_ARCH=75 -DUSE_DIAQ=1 -DDIAQ_INCLUDE_DIR=<path_to_diaq>/include -DDIAQ_LIB_DIR=<path_to_diaq>/build/lib .. && make -j 4
# sanity check the build with DIAQ integrations
$ ./qasm/nwq_qasm -q ../data/benchmarks/ghz/ghz22.qasm -backend DIAQ_OpenMP -sim sv -metrics
\end{lstlisting}

\textbf{3) Benchmarks:}
The benchmarks repository contains Jupyter notebooks and Python scripts for generating plots and performing additional analysis of quantum circuits and their sparsity. The prerequisites include a virtual environment with python $\geq$ 3.8 and most Python packages from requirements.txt installed. The following steps illustrate the setup and usage:

\begin{lstlisting}[frame=single, basicstyle=\small\ttfamily, breaklines=true]
$ python3.8 -m venv qsparseVirtEnv
$ source qsparseVirtEnv/bin/activate
$ pip install -r <benchmarks_dir>/requirements.txt
\end{lstlisting}

The \texttt{\seqsplit{/analysis/jupyter\_notebooks}} directory contains code for obtaining timesteps in SupermarQ circuits and performing sparsity analysis. The resulting images are saved in the \texttt{\seqsplit{/analysis/images}} directory (Figures 1(c), 2, 3). The \texttt{\seqsplit{/analysis/superMarQ\_benchmarks.ipynb}} notebook contains the analysis of SupermarQ benchmarks GHZ, HAM, and Mermin-Bell (Figures 1(a), 1(b) in the paper).

\begin{lstlisting}[frame=single, basicstyle=\small\ttfamily, breaklines=true]
# raw_data for Figure 4
$ cd benchmarks/bench
$ python format_bench.py all 1
\end{lstlisting}

The \texttt{\seqsplit{analysis/jupyter\_notebooks/memory\_savings\_analysis.ipynb}} notebook contains the code to generate the memory savings plot (Figure 4 in the paper). The \texttt{\seqsplit{nwq\_sim/raw\_results}} directory contains the raw results of the qasmbench and SupermarQ benchmark runs with NWQ-Sim/SV-Sim with and without DiaQ integrations. The \texttt{\seqsplit{nwq\_sim/jupyter\_notebooks/supermarq\_analysis.ipynb}} notebook contains the code to generate the SupermarQ analysis plots (Figures 5, 7). The \texttt{\seqsplit{nwq\_sim/jupyter\_notebooks/qasmbench\_analysis.ipynb}} notebook contains the code to generate the qasmbench analysis plot (Figure 8).
